# Supplementary material for: MixHop: Higher-Order Graph Convolutional Architectures via Sparsified Neighborhood Mixing
Source: arXiv:1905.00067 source file (2019-06-19)
Supplement: Supplementary file 1 [file appendix.tex]

\newpage

\appendix

\section{Synthetic Dataset}
For generating synthetic data, we split nodes to equal size classes $1, 2, ..., k$. At each iteration, we add new node $v$ with a random class to the graph. The probability of connecting $v$ to existing node $u$ is the following:
\begin{itemize}[itemsep=-3pt,topsep=-3pt]
    \item if $c_v = c_u$: $p_{v \rightarrow u} = d_u \times homophily$
    \item if $c_v \neq c_u$: $p_{v \rightarrow u} = d_u \times homophily \times w_{|c_v - c_v|}$
\end{itemize}

Where $c_v$ is class of node $v$ and $w_{|c_v - c_v|}$ is weight of connecting two different classes with \textit{distance} $|c_v - c_u|$. By \textit{distance} we mean shortest distance of two classes on a circle, starting from class $1$ to $k$ respectively. The weight is exponentially decreasing with increasing of \textit{distance}. For example if we have $6$ classes and $w_{|1 - 4|} = 1$, then $w_{|1 - 3|} = w_{|1 - 5|} = 2$ and $w_{|1 - 2|} = w_{|1 - 6|} = 4$. We normalize $w$ such that $\sum w_i = 1$. We use $k=10$.

The final probability of connecting $v$ to $u$ is normalized over all existing nodes: $p_{v \rightarrow u} =\frac{p_{v \rightarrow u}}{\sum_i p_{v \rightarrow i}}$. Since $\sum w_i = 1$, based on \cite{karimi}, sampling edges proportional to $p_{v \rightarrow u}$ at each iteration, would give us a graph with desired homophily and Barabasi-Albert degree distribution. Figure \ref{fig:synthetic}, shows two graphs with same number of nodes and edges, but with different homophily coefficients. As expected, edges of \ref{fig:synthetic_h1} are between different classes, while the edges of \ref{fig:synthetic_h9} are within classes. 

\begin{figure}[h]
    \centering
    \begin{subfigure}[t]{0.48\columnwidth}
        \centering
        \includegraphics[width=\columnwidth]{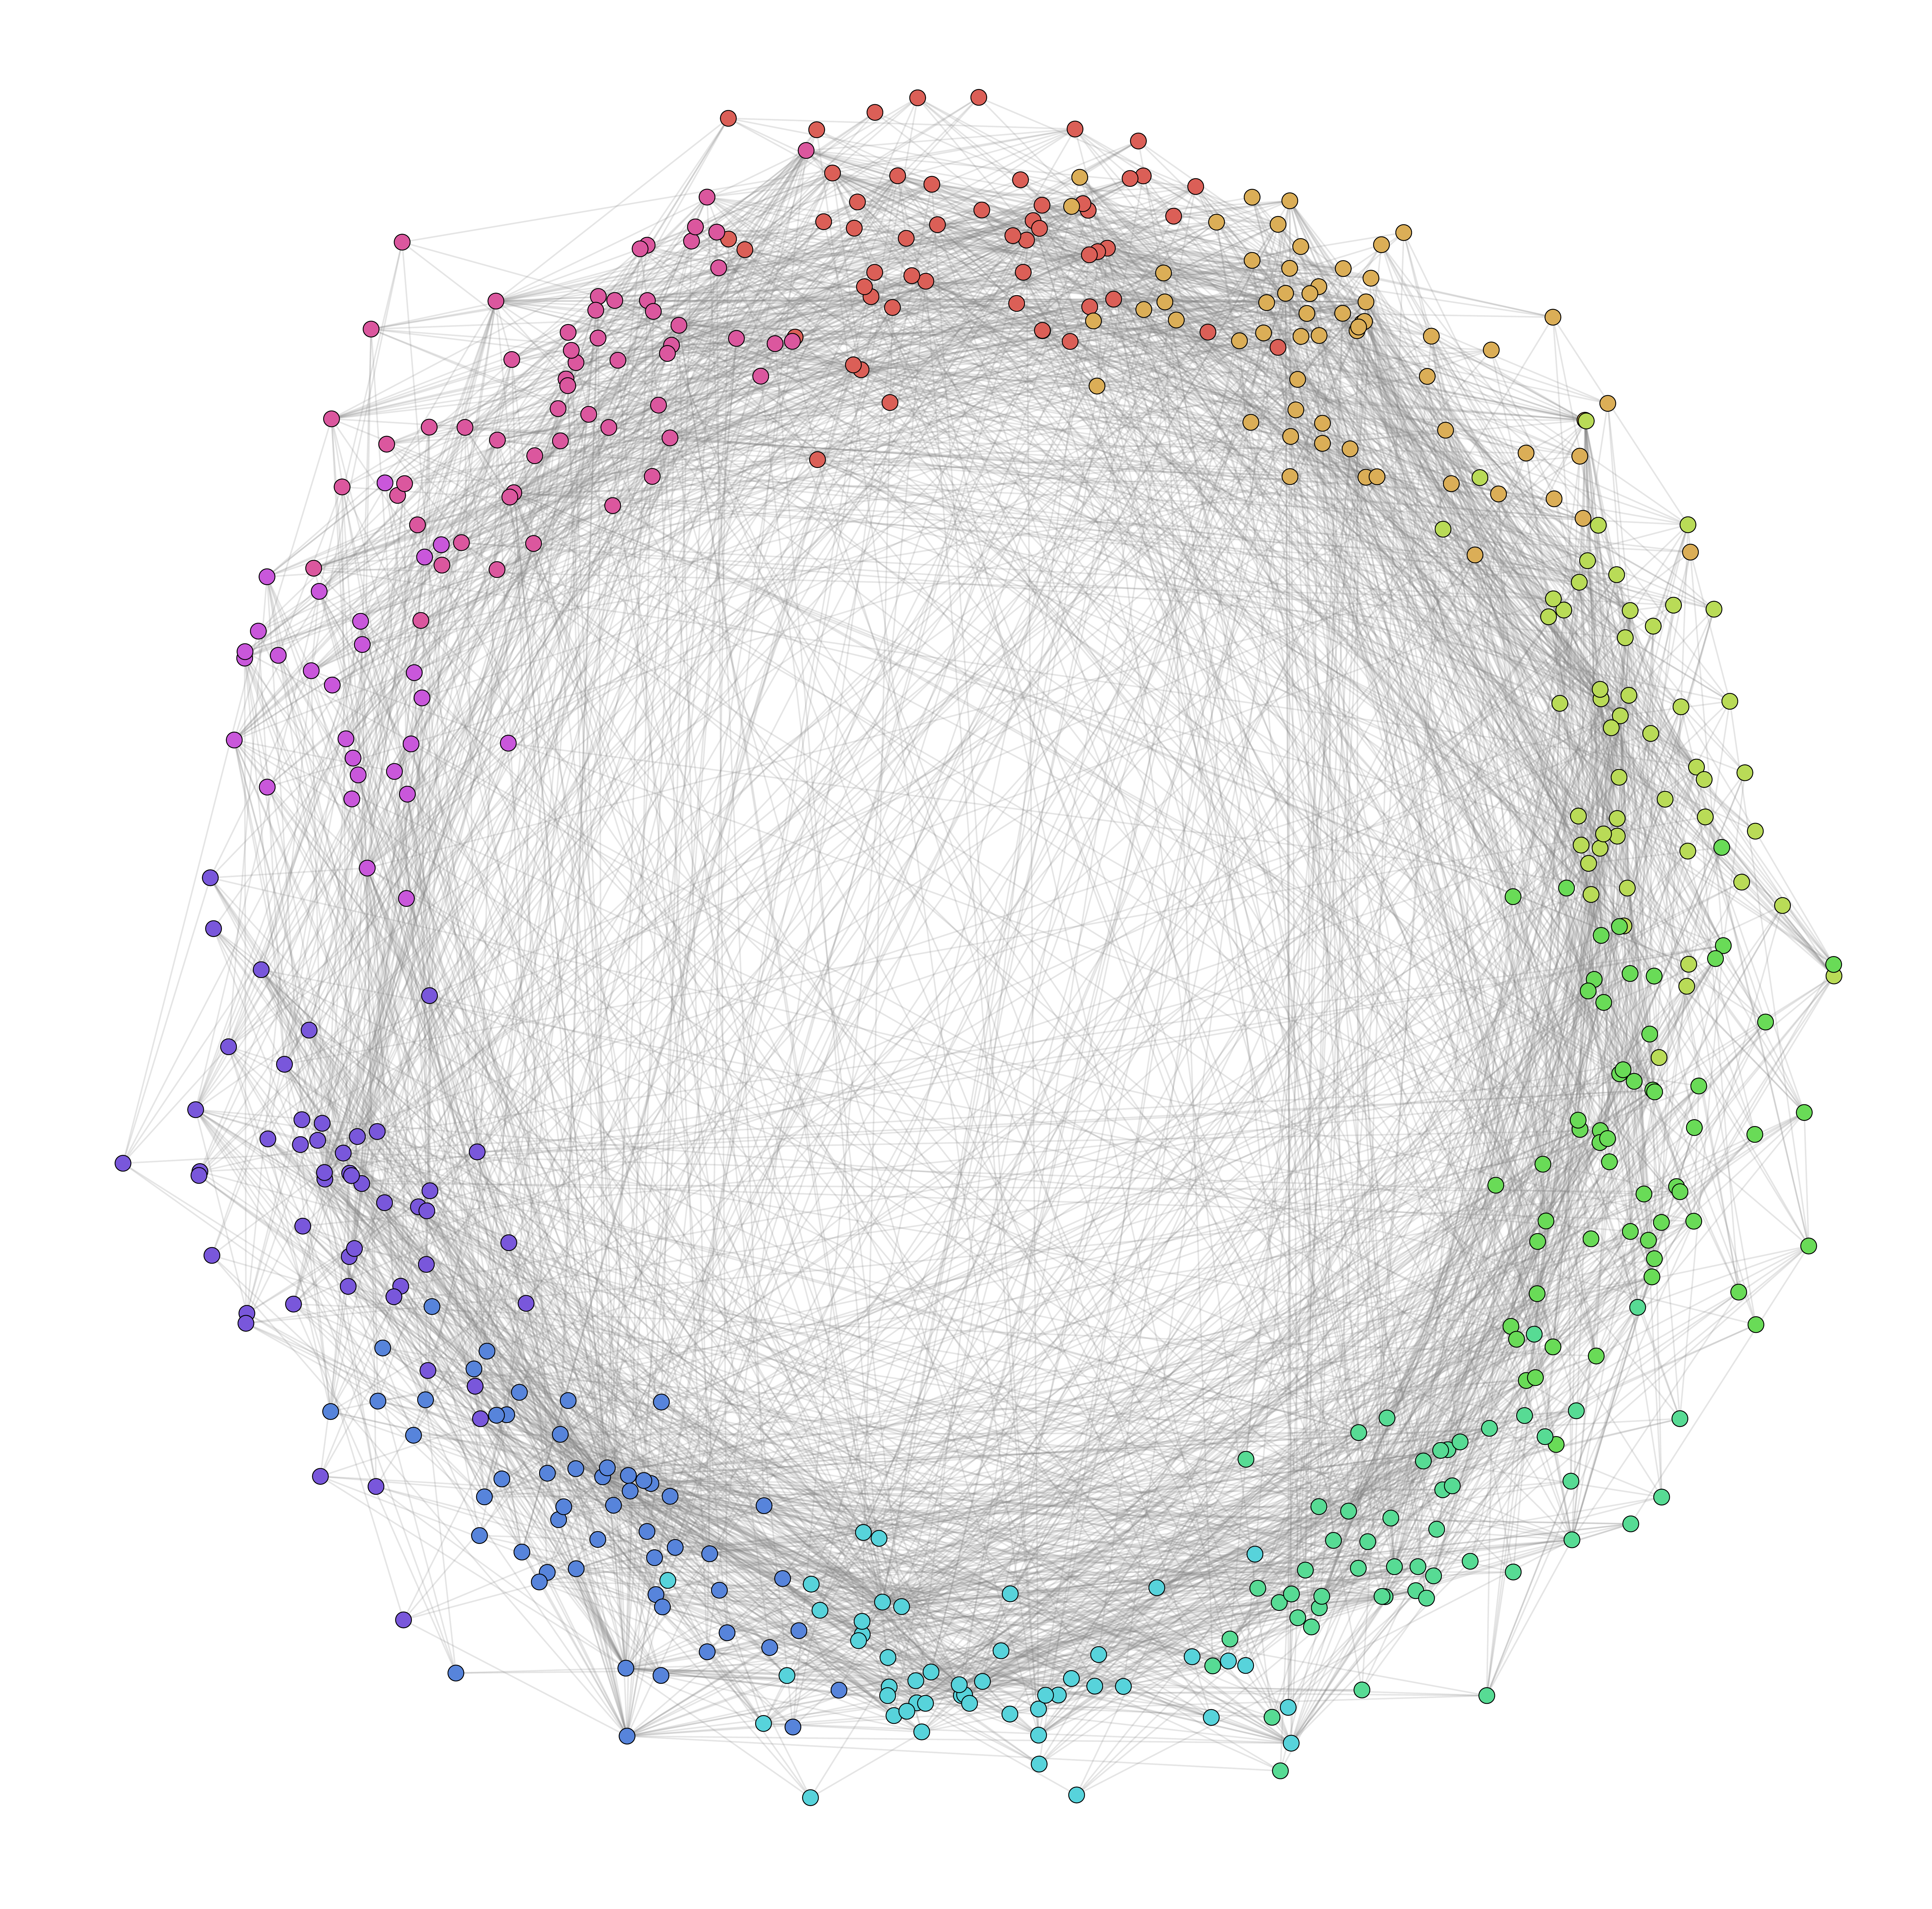}
        \caption{Homophily = 0.1}\label{fig:synthetic_h1}
    \end{subfigure}
    \begin{subfigure}[t]{0.48\columnwidth}
        \centering
        \includegraphics[width=\columnwidth]{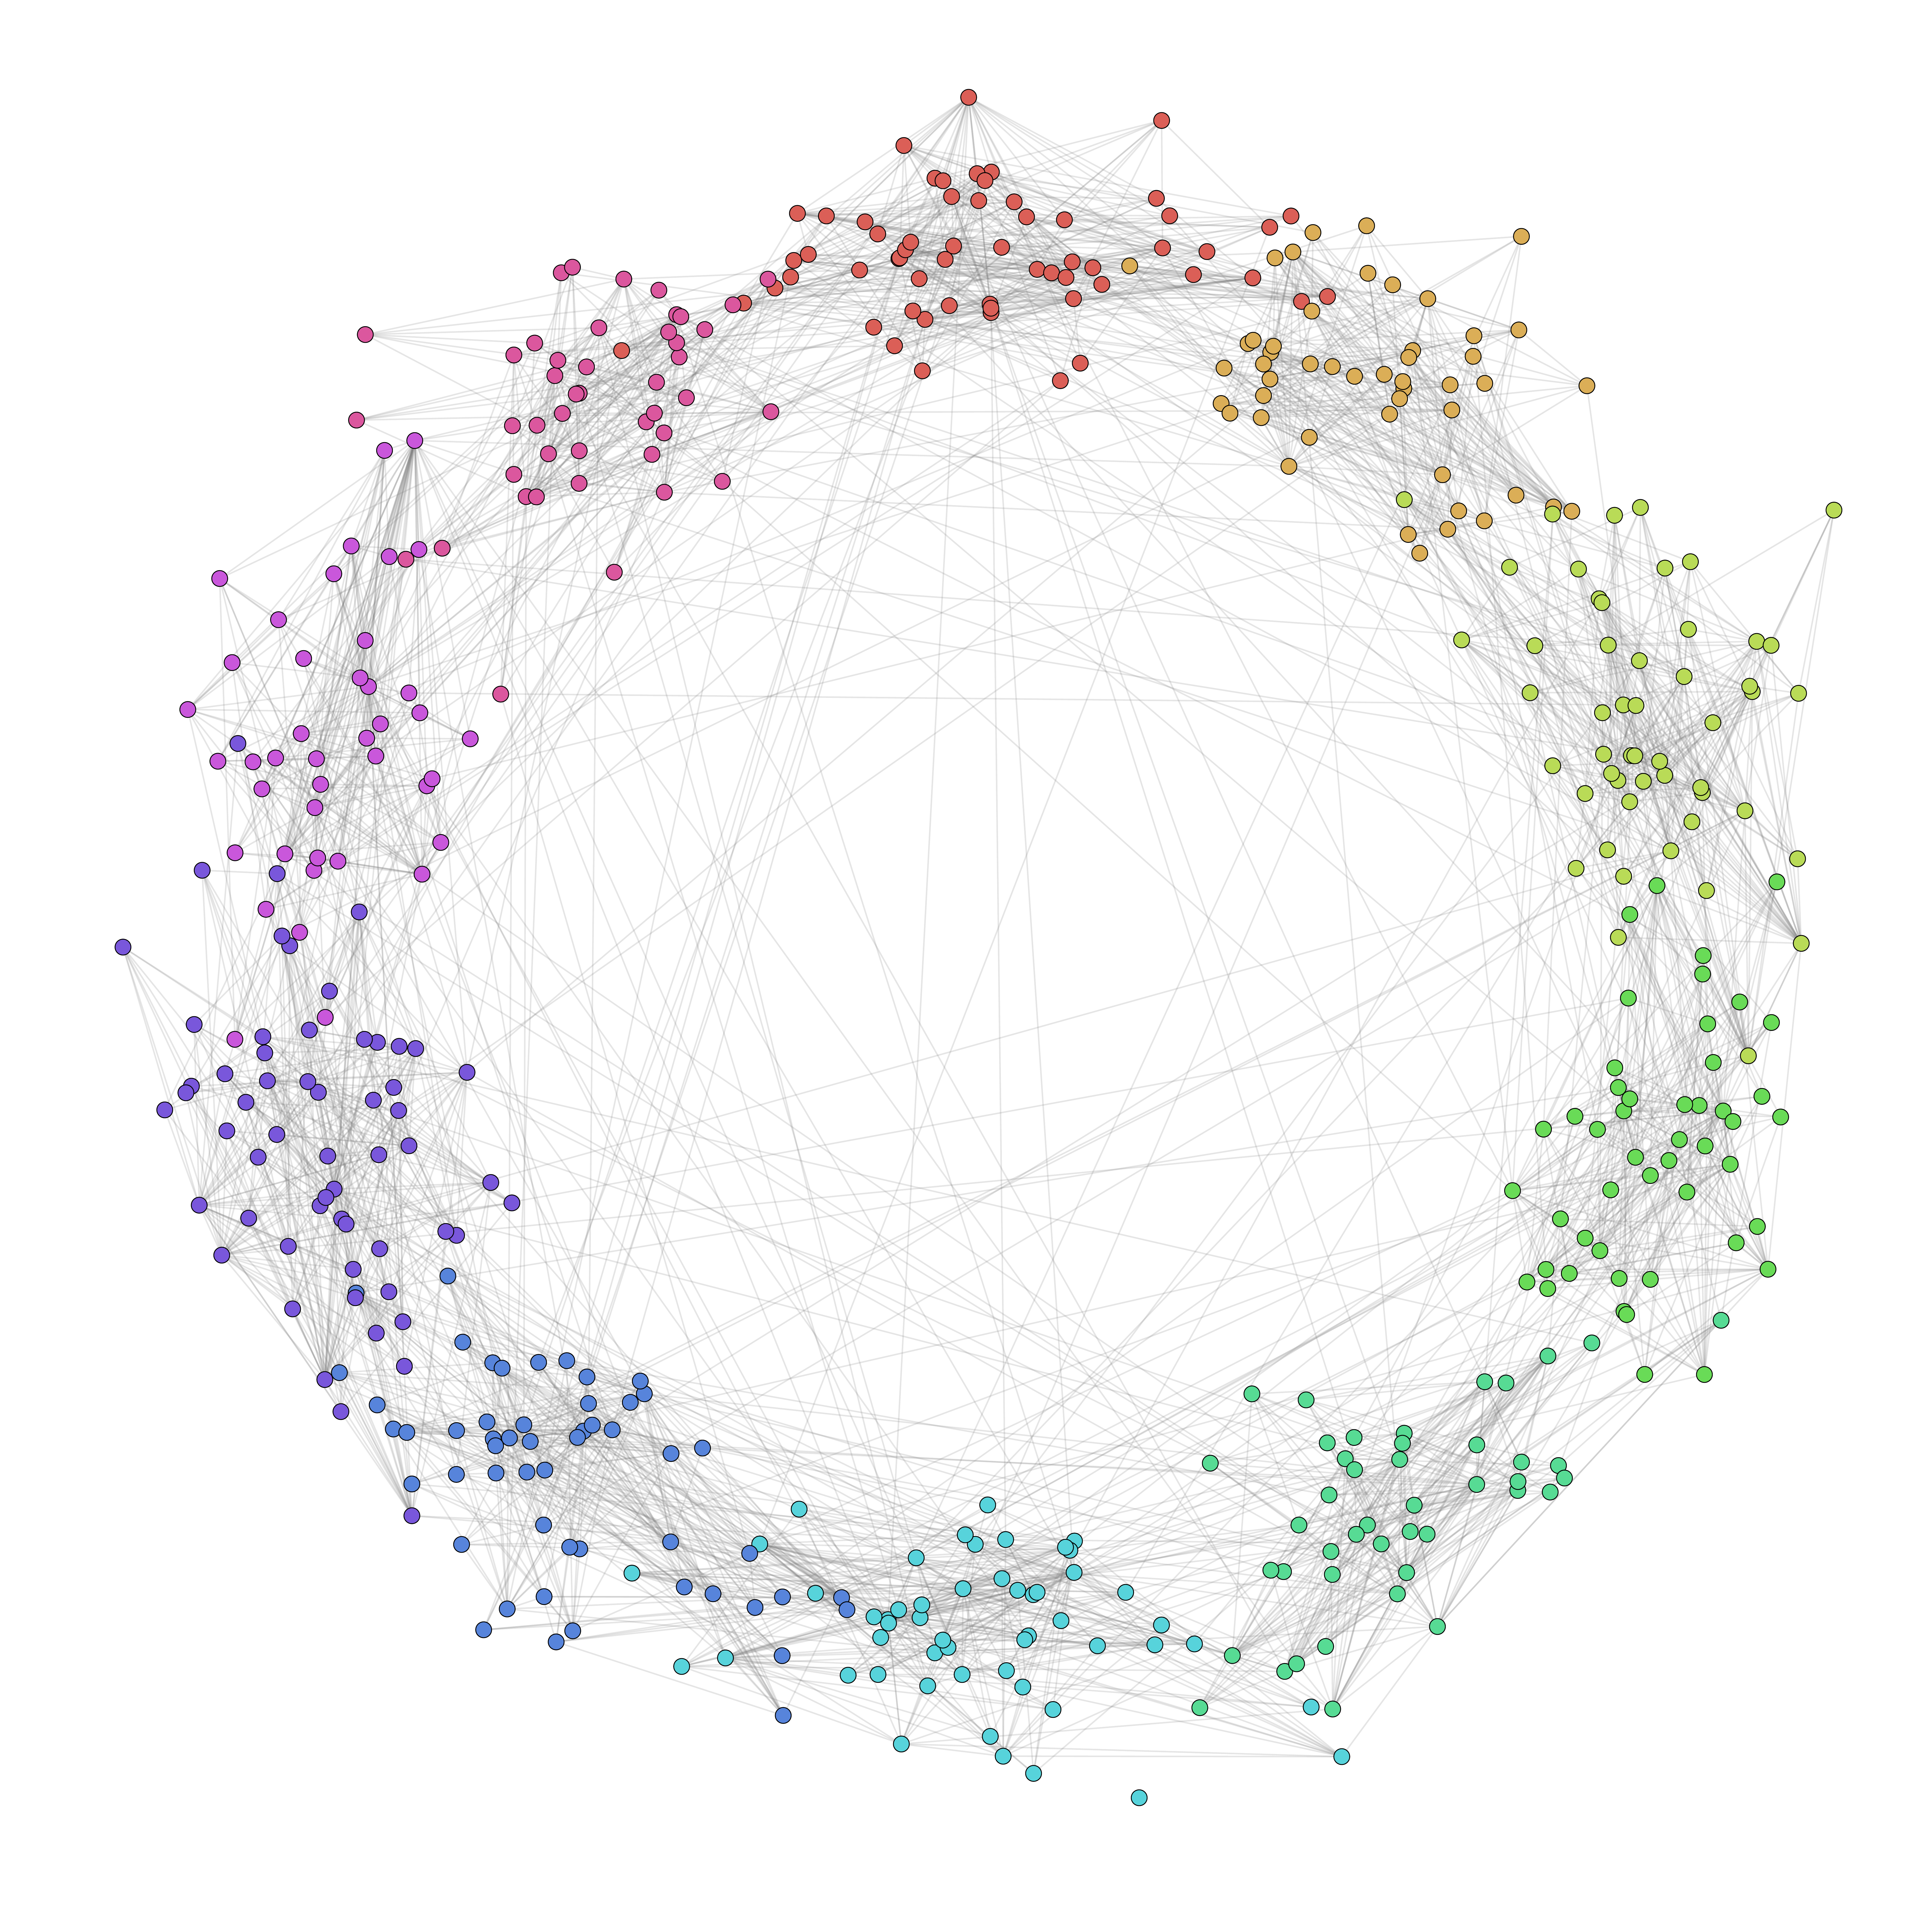}
        \caption{Homophily = 0.9}\label{fig:synthetic_h9}
    \end{subfigure}
     
    \caption{Synthetic data generated for (a) $homophily=0.1$ and (b) $homophily=0.9$. Both graphs have $500$ nodes, $2798$ edges and $10$ equal size classes. Classes are specified with different color of node. \label{fig:synthetic}}
\end{figure}

The feature values of the nodes are sampled from 2D Gaussians. In particular, each node class has its own Gaussian. The means of the Gaussians can be best described in polar coordinates: Each mean has radius 300 and angle $\frac{2 \pi}{10} \times \textrm{(class id)}$. The covariance matrix of each class is $3500 \times \textrm{diag}([7, 2])$, that is rotated by angle $\frac{2 \pi}{10} \times \textrm{(class id)}$. The synthetic datasets are available for download via \href{https://github.com/samihaija/mixhop/tree/master/data/synthetic}{github}.

\section{Future Work}
Because our work has general applicability to a large number of graph tasks, we believe there is significant room to fine tune our model. 
In the spirit of \citet{sage}, we can extend our methods to large graphs (e.g. with millions of edges) that might not fit in computer memory. Such scalability would be vital for the practical usage of these methods.
In this work, we utilize a weighted softmax output layer that acts as a regularization method on the final feature output of the model. We believe that different kinds of output layers may be better suited for different tasks. An easy extension of our work is to analyze how our model performs with a fully connected output layer. Similarly, to apply our model to graph classification, one can average all node representations at the output layer (e.g. using a set2set model) to feed into classification layers for the full graph.
While we analyze the ability of our model to learn delta operators in this work, we think that it would be fascinating to visualize how each delta operator actually operates in the graph. Specifically, we want to observe which community edges the model is capturing. In future experiments, we hope to explore methods of visualizing these features.
